# Supplementary material for: Gradient Coreset for Federated Learning
Source: arXiv:2401.06989 source file (2024-01-13)
Supplement: Supplementary file 1 [file appendix.tex]

\section{Code}
We have released anonymized code at the URL: \url{https://anonymous.4open.science/r/GM_Federated-498F}

\section{Notation}

To improve readability we list the various notations used and their meaning in table \ref{tab:notations}.

\begin{table}[h]
    \centering
    %\resizebox{0.9\textwidth}{!}{
    \begin{tabular}{c l}
    \hline
       Notation & Description\\ \hline \\
       $\cliset$ & Set of clients $\{c_1,c_2,\cdots, c_N\}$ \\
       $N$ & No. of clients \\
       $D_T$ & Training data partitioned across $N$ clients i.e. $\trndata = \bigcup_{i=1}^N D_i$ \\
       $D_i$ & Data at each client\\
       $\valdata$ & Server's data \\
       $\coreset$ & Subset selected at client $i$ on round $t$ \\
        $\serverloss$ &  Server loss computed on $\valdata$ \\
       $\cliloss$ & Loss at each client \\
       $\avgcliloss(\param)$ &  Average loss of clients i.e. $\sum_{i=1}^N \cliloss(\param)$ \\
       $E$ & Denotes the number of local gradient update steps that the client  performs \\
       %$N$ & No. of clients \\
       %$N$ & No. of clients \\
        \hline
    \end{tabular}%}
    \caption{ Important Notations and Descriptions} 
    \label{tab:notations}
\end{table}

\section{Complete algorithm of \model{}}
We refer the reader to Algorithm \ref{alg:greedy} for a complete pseudocode for \model{}.
\begin{figure} [H]
    \centering
    \begin{minipage}{0.6\textwidth}
        \begin{algorithm}[H] 
        \caption{\model{} algorithm~\label{alg}}
        \label{alg:greedy}
        \begin{algorithmic}[1]
        \REQUIRE \small{ Clients $\mathcal{C} = \{c_1, \cdots, c_N\}$, Server $\mathcal{S}$, Training Data $D_i = \{(x_{ij}, y_{ij})_{j=1}^{n_i}\}_{i=1}^N$, Server Data $\valdata$, communication rounds $T$, budget $b$, number of clients per round $m$, local and global learning rates $\eta_l, \eta_g$, , local gradient steps $E$, server broadscast round $K$}
            \STATE $\theta_0 \leftarrow \textsc{init\_}\flmdl$; \;\;$\Xcal_i^0 \leftarrow \textsc{init\_random\_samples}(i) \;\; \forall i \in [N]$
              \FOR{round $t \in [T]$}
                    \STATE \textbf{server does:}
                    \STATE $S^t \leftarrow$ sample $m$ out of $N$ clients
                    % \IF{$t \% K == 0$}
                        \STATE Broadcast ($\theta^t, \nabla_\theta \serverloss(\theta^t)$) to $S^t$ if {$t \% K = 0$ else Broadcast $\theta^t$ to $S^t$
                    % \ELSE
                        % \STATE broadcast $\theta^t$ to $S^t$
                    % \ENDIF
                    \STATE \textbf{each client $c_i \in S^t$ does:}
                     % \IF{$t \% K == 0$}
                        \STATE $\coreset \leftarrow $  solve obj. ~\eqref{eq:gmobj} using greedy algorithm if $t \% K = 0$ else  $\Xcal_i^{t-1}$
                    % \ELSE
                        % \STATE $\coreset = \Xcal_i^{t-1}$
                    % \ENDIF
                    \STATE Set $\theta^{'} \leftarrow \theta^t$
                    \FOR{$e \in [E]$}
                        \STATE sample a mini-batch $\Bcal \overset{\iid}{\sim} \coreset$
                        \STATE $\theta^{'} \leftarrow \theta^{'} - \eta_l \frac{1}{|\Bcal|}\sum_{(x, y) \in \Bcal}\cliloss(f_{\theta^{'}}(x), y)$
                    \ENDFOR 
                    \STATE Broadcast $\delta_i^t \leftarrow \theta^t - \theta^{'}$ to $\mathcal{S}$
                    
                    \STATE \textbf{server does:}
                    \STATE $\theta^{t+1} \leftarrow \theta^t + \eta_g \sum_{i \in S^t} \delta_i^t$
              \ENDFOR
            \RETURN $f_{\theta^T}$
        \end{algorithmic}
        \end{algorithm}
    \end{minipage}
\end{figure}

\section{Convergence Proof}

Our proof technique is inspired partly from  \citep{scaffold}.

\subsection{Additional definitions}

\textbf{(A1)}  Let the loss functions of clients be denoted as $\{\cliloss\}_{i=1}^N$ and let $\serverloss$ denote the server loss computed on $\valdata$. We assume that the client and the server losses are convex. Let $\paramstar = \text{argmin}_{\param} \serverloss(\param)$ denote the optimal parameters w.r.t the server loss. We assume a  bound on the dissimilarity between clients' gradient and the validation gradient at the server with the following inequality

%\textcolor{red}{To profs: Is the below assumption reasonable?} \todo{Since we have an elegant assumption concerning the data at $S$, that is it is label noise-free and also it privacy protected, (i) we have freedom in constructing such an $S$ which is noise free (ii) But can we provide some recipe - such as clients with very very small FL budget in the zeroth budget at each client and clients pass this small FL based coreset to the server as $S$. Honestly, a private $S$ is an opportunity for nice recipes but without a recipe for $S$, we might irk some reviewer. }
\begin{equation}
    \begin{aligned}
        \frac{1}{N}\sum_{i=1}^{N}\|\nabla \cliloss(\param)\|^2 \leq G^2 + 2\beta B^2 (\avgcliloss(\param)-\serverloss^{*}) \text{ where }\serverloss^{*} = \serverloss(\paramstar)
    \label{grad_dis2}
    \end{aligned}
\end{equation}

where $G$ and $B$ are constants such that $G \geq 0, B \geq 1$ and $\avgcliloss(\param) = \sum_{i=1}^N \cliloss(\param)$

\textbf{(A2)} If $\cliloss$ is $\mu$-convex for $\mu \geq 0 $ then we have:

$$\langle \nabla \cliloss(\param), \paramprime - \param\rangle \leq -\bigg(\cliloss(\param) - \cliloss(\paramprime) + \frac{\mu}{2}\|\param-\paramprime\|^2 \bigg) \forall i,\param,\paramprime$$
%\text{, for any } 

\textbf{(A3)} For a given coreset $\coreset \subseteq D_i$, let $\clilossgm$ denote the client's loss function on $\coreset$.  Then $\cligradfun(\param)$  be an  unbiased stochastic gradient of $\clilossgm$ with \textit{bounded variance}

$$\mathbb{E}_{\coreset}||\cligradfun(\param) - \nabla \clilossgm(\param)||^2 \leq \sigma^2 \;\; \forall i,\param$$ 

Note that (A3) only bounds the variance within the same client, but not the variance across the clients.

\textbf{(A4)} Each client loss function $\cliloss$ are $\beta$-smooth and satisfy:

$$||\nabla \cliloss(\param) -  \nabla \cliloss(\paramprime)|| \leq \beta||\param - \paramprime|| \text{, for any } i,\param, \paramprime$$

The assumption (A4) also implies the following quadratic upper bound on $\cliloss$,

$$\cliloss(\paramprime) \leq \cliloss(\param) + \langle \nabla \cliloss(\param),\paramprime- \param\rangle + \frac{\beta}{2}||\param - \paramprime||^2$$

We can also express the smoothness constraint as: (via \cite{nesterov2018lectures}, Theorem 2.1.5)

$$\frac{1}{2\beta N} \sum_{i=1}^{N}||\nabla \cliloss(\param) -  \nabla \cliloss(\paramstar)|| \leq \avgcliloss(\param) - \avgcliloss(\paramstar)$$ \\

where $\avgcliloss(\param) = \sum_{i=1}^N \cliloss(\param)$

% Further, if $\cliloss$ is twice-differentiable, (A4) implies that $||\nabla^2 \cliloss(\param) \leq \beta$  for any \param.

\subsection{Some technical lemmas}
\begin{lemma} (perturbed strong convexity) The following holds for any $\beta$-smooth and $\mu$-strongly convex function $h$, and any $\param, \paramprime, \parampprime$ in the domain of $h$:

$$\langle \nabla h(\param),\parampprime - \paramprime\rangle \geq h(\parampprime) - h(\paramprime) + \frac{\mu}{4}\|\paramprime-\parampprime\|^2 - \beta\|\parampprime-\param\|^2$$
\label{convex}
\end{lemma}

\begin{lemma} (separating mean and variance). Let $\{\mathsf{\Xi}_1, . . . , \mathsf{\Xi}_{\tau} \}$ be $\tau$ random variables in $\mathbb{R}^d$ which are not necessarily independent. First suppose that their mean is $\mathbb{E}[\mathsf{\Xi}_i] = \xi_i$ and variance is bounded as $\mathbb{E}[\|\mathsf{\Xi}_i - \xi_i\|^2] \leq \sigma^2 $. Then, the following holds

$$\mathbb{E}[\|\sum_{i=1}^{\tau} \mathsf{\Xi}_i\|] \leq  \mathbb{E}[\|\sum_{i=1}^{\tau} \xi_i\|^2] +  \tau^2 \sigma^2 $$

% Now instead suppose that their conditional mean is $\mathbb{E}[\mathsf{\Xi}_i|\mathsf{\Xi}_{i-1},. . . , \mathsf{\Xi_1}] = \xi_i$i.e. the variables $\{\mathsf{\Xi}_i - \xi_i\}$ form a martingale difference sequence, and the variance is bounded by $\mathbb{E}[\|\mathsf{\Xi}_i - \xi_i\|^2] \leq \sigma^2 $ as before. Then we can show the tighter bound
% $$\mathbb{E}[\|\sum_{i=1}^{\tau} \mathsf{\Xi}_i\|] \leq  2\mathbb{E}[\|\sum_{i=1}^{\tau} \xi_i\|^2] +  2\tau \sigma^2$$
\label{sep_mean}
\end{lemma}

\begin{lemma}  (relaxed triangle inequality). Let ${v_1, . . . , v_{\tau} }$ be $\tau$ vectors in $\mathbb{R}^d$. Then the following is true:
\begin{align}
    \|v_i + v_j\|^2 \leq (1+a)\|v_i\|^2 + (1+\frac{1}{a})\|v_j\|^2 \text{ for any } a > 0
    % \item $\|\sum_{i=1}^{\tau}v_i\|^2 \leq \tau \sum_{i=1}^{\tau}\|v_i\|^2$
\label{relax_tri}    
\end{align}
\end{lemma}

%\label{lem_one}
\begin{theorem}  (one round progress) For any client $i$ and subset size or budget $b > 0$, n size of the coreset, let $\mbox{E}_\lambda(\mathbf{w}_i^t, \Xcal_i^t)$ from  \eqref{eq:gmobj} be bounded as, 

\begin{align}
     \min_{\mathbf{w}} \mbox{E}_\lambda(\mathbf{w}, \Xcal_i^t)  = \min_{\mathbf{w}} \bigg \{ \lambda \lVert \mathbf{w} \rVert^2 + {\big\Vert \sum_{j \in \Xcal_i^t} \mathbf{w}_{j} \nabla_{\theta}\ell_i^j(\theta^t) -  \nabla_{\theta}\serverloss (\theta^t)\big\Vert} \bigg \} \nonumber
     \leq \epsilon_i(b) \nonumber
\end{align}

where, 

\begin{align}
      \epsilon_i(b) = \max_{\Xcal \in D_i^b} \min_{\mathbf{w}} \mbox{E}_\lambda(\mathbf{w}, \Xcal)  \nonumber
\end{align}

where $D_i^b$ is the set of all subsets of size $b$. Thus, $\epsilon_i(b)$  denotes the max error in approximating the server's loss gradient $\nabla\serverloss$ using a any subset of budget $b$ at client $i$. Let

\begin{align}
     \epsilon_{max} = \max_{i \in [N]} {\epsilon_i(b)}
     \label{grad_err2}
\end{align}

bound the maximum coreset selection error across clients. Suppose our loss functions $\{\cliloss\}$ and $\serverloss$ satisfies assumptions (A1) - (A4). For any step-size satisfying $\eta_l \leq \frac{1}{(1+B^2)72\beta E\eta_g}$ with effective step-size is $\tilde{\eta} := E\eta_g\eta_l$, the updates of any subset selection algorithm would at round $t$ satisfy 

\begin{equation}
\begin{aligned}
\mathbb{E}||\param^t -\serveroptparam||^2  & = \bigg( 1- \frac{\mu \tilde{\eta}}{2} \bigg)||\param^t - \serveroptparam||^2 +   2\tilde{\eta}\epsilon_{max} ||\param^t - \serveroptparam|| - (2\tilde{\eta} - 16 \tilde{\eta}^2\beta(B^2+1))(\avgcliloss(\param^t) - \serverloss(\serveroptparam)) \\ 
&+ (1+2\tilde{\eta}\beta)2 \tilde{\eta}\beta \mathcal{E}_t + \bigg( 1 - \frac{S}{N}\bigg)\frac{8\tilde{\eta}^2}{S}G^2 +2\tilde{\eta}^2\epsilon_{max}^2 +\tilde{\eta}^2\sigma^2
\end{aligned}
\end{equation}
%\label{lem_one}

where $\mathcal{E}_t$ is the drift caused by the local updates on the clients defined as

$$\mathcal{E}_t := \frac{1}{EN}\sum_{k=1}^E \sum_{n=1}^N \mathbb{E}_{t}||\param^t_{i,k-1} - \param^{t-1}||^2 $$

and $\serveroptparam = \text{argmin}_{\theta}\serverloss(\theta)$. $\param^t_{i,k}$ denotes the parameters of the model after $k^{th}$ local update of the $i^{th}$ client.

\end{theorem}
\begin{proof}

Let $\cligradfun(\param)$ be unbiased stochastic gradient of $\nabla \clilossgm$ at $\param$. Then the update shared by the client to server is,

\begin{equation}
    \begin{aligned}
        \Delta \param = -\frac{\tilde{\eta}}{EN}\sum_{k,i} \cligradfun (\param_{i,k-1}) \hspace{1em} \text{ and } \hspace{1em}
        \mathbb{E}[\Delta \param] = -\frac{\tilde{\eta}}{EN}\sum_{k,i}\nabla \clilossgm(\param_{i,k-1})
    \end{aligned}
\end{equation}

Adding and subtracting $\nabla \cliloss(\param_{i,k-1})$,

\begin{equation}
    \begin{aligned}
        \mathbb{E}[\Delta \param] = -\frac{\tilde{\eta}}{EN}\sum_{k,i}( \cligradfun(\param_{i,k-1}) + \nabla \cliloss(\param_{i,k-1}) - \nabla \cliloss(\param_{i,k-1}))
    \end{aligned}
\end{equation}

Now,
\begin{multline}
\mathbb{E}_{t-1}||\param + \Delta \param -\serveroptparam||^2   =  ||\param - \serveroptparam||^2
+ \frac{2\tilde{\eta}}{EN}\sum_{k,i}\langle \nabla \cliloss(\param_{i,k-1}),\serveroptparam - \param \rangle \\
 + \frac{2\tilde{\eta}}{EN}\sum_{k,i}\langle \nabla \cliloss(\param_{i,k-1}) -   \cligradfun(\param_{i,k-1}),\param - \serveroptparam\rangle
+\tilde{\eta}^2 \mathbb{E}_{t-1}\bigg\|\frac{1}{ES}\sum_{k,i\in S}   \cligradfun(\param_{i,k-1})\bigg\|^2
\label{eq_con1}
\end{multline}

Using Cauchy–Schwarz inequality, 

\begin{multline}
\mathbb{E}_{t-1}||\param+\Delta \param -\serveroptparam||^2   \leq  ||\param - \serveroptparam||^2
+ \frac{2\tilde{\eta}}{EN}\sum_{k,i}\langle \nabla \cliloss(\param_{i,k-1}),\param - \serveroptparam\rangle \\
 + \frac{2\tilde{\eta}}{EN}\sum_{k,i}\big\|  \cligradfun(\param_{i,k-1}) - \nabla \cliloss(\param_{i,k-1})\big\|.\big\|\param - \serveroptparam\big\|
+\tilde{\eta}^2 \mathbb{E}_{t-1}\bigg\|\frac{1}{ES}\sum_{k,i\in S}   \cligradfun(\param_{i,k-1})\bigg\|^2
\label{eq_con1}
\end{multline}

Applying Eq. \ref{grad_err2},

\begin{multline}
\mathbb{E}_{t-1}||\param+\Delta \param - \serveroptparam||^2  \leq  ||\param - \serveroptparam||^2
+ \frac{2\tilde{\eta}}{EN}\sum_{k,i}\langle \nabla \cliloss(\param_{i,k-1}),\param - \serveroptparam\rangle 
 + 2\tilde{\eta}\epsilon_{max}\big\|\param - \serveroptparam\big\| \\
 +\tilde{\eta}^2 \mathbb{E}_{t-1}\bigg\|\frac{1}{ES}\sum_{k,i\in S}   \cligradfun(\param_{i,k-1})\bigg\|^2
\label{eq_con1}
\end{multline}

as $E_{\lambda}(\Xcal_i^k) \leq \epsilon_{max}$, therefore  $\big\| \nabla \clilossgm (\param_{i,k}) -\nabla \cliloss (\param_{i,k}) \big\|^2 \leq \epsilon_{max}$ as $\lambda ||\corewt_i|| ^2 > 0$. Upon applying \textbf{Lemma \ref{sep_mean}} on Eq.\ref{eq_con1} using the assumption $A2$,

\begin{equation}
\begin{aligned}
\mathbb{E}_{t-1}||\param + \Delta\param -\serveroptparam||^2  & = ||\param - \serveroptparam||^2 + \underbrace{\frac{2\tilde{\eta}}{EN}\sum_{k,i}\langle \nabla \cliloss(\param_{i,k-1}),\param - \serveroptparam\rangle}_\text{$\Acal$1} \\ &+\underbrace{\tilde{\eta}^2 \mathbb{E}_{t-1}\bigg\|\frac{1}{ES}\sum_{k,i\in S}\nabla \clilossgm(\param_{i,k-1})\bigg\|^2}_\text{$\Acal$2} +\tilde{\eta}^2\sigma^2 + 2\tilde{\eta}\epsilon_{max}\big\|\param - \serveroptparam\big\|
\label{eq_con2}
\end{aligned}
\end{equation}

We can directly apply Lemma \ref{convex} with $h = \cliloss, \param = \param_{i,k-1}, \paramprime = \serveroptparam\text{ and }\parampprime = \param$ to the first term $\Acal$1

\begin{equation}
\begin{aligned}
\Acal1 & = \frac{2\tilde{\eta}}{EN}\sum_{k,i}\langle \nabla \cliloss(\param_{i,k-1}),\param - \serveroptparam\rangle\\
& \leq \frac{2\tilde{\eta}}{EN}\sum_{k,i}\Big(\cliloss(\param) - \cliloss(\serveroptparam) + \beta\|\param_{i,k-1}-\param\|^2 - \frac{\mu}{4}\|\param-\serveroptparam\|^2  \Big) \\
& = -2\tilde{\eta} \Big( \avgcliloss(\param) - \avgcliloss(\serveroptparam) + \frac{\mu}{4}\|\param-\serveroptparam\|^2\Big)  + 2\beta\tilde{\eta} \mathcal{E}_t \\
& \leq - 2\tilde{\eta} \Big( \avgcliloss(\param) - \serverloss(\serveroptparam) + \frac{\mu}{4}\|\param-\serveroptparam\|^2\Big)  + 2\beta\tilde{\eta} \mathcal{E}_t
\end{aligned}
\end{equation}

The last step follows when server loss at optimal parameter is less than average loss client loss evaluated at optimal parameter for server loss. 
%\textcolor{red}{Can we assume in the last step follows because we have $\serverloss(\serveroptparam) \leq \avgcliloss(\serveroptparam)$}
%\todo{Again this is intuitive since $S$ can be constructed to be noise free and can be constructed by us! Since we have an elegant assumption concerning the data at $S$, that is it is label noise-free and also it privacy protected, (i) we have freedom in constructing such an $S$ which is noise free (ii) But can we provide some recipe - such as clients with very very small FL budget in the zeroth budget at each client and clients pass this small FL based coreset to the server as $S$. Honestly, a private $S$ is an opportunity for nice recipes but without a recipe for $S$, we might irk some reviewer. }
For the second term A2, we repeatedly apply the relaxed triangle inequality with $a=1$ (Lemma \ref{relax_tri})

\begin{equation}
\begin{aligned}
\Acal2 & = \tilde{\eta}^2 \mathbb{E}_{t-1}\bigg\|\frac{1}{ES}\sum_{k,i\in S}\nabla \clilossgm(\param_{i,k-1}) + \nabla \cliloss(\param_{i,k-1}) - \nabla \cliloss(\param_{i,k-1})\bigg\|^2\\
& \leq  2 \tilde{\eta}^2 \mathbb{E}_{t-1}\bigg\|\frac{1}{ES}\sum_{k,i\in S} \nabla \cliloss(\param_{i,k-1})\bigg\|^2 + 2 \tilde{\eta}^2 \mathbb{E}_{t-1}\bigg\| \frac{1}{ES}\sum_{k,i\in S}\nabla \clilossgm(\param_{i,k-1})  - \nabla \cliloss(\param_{i,k-1})\bigg\|^2\\
& \leq  2 \tilde{\eta}^2 \mathbb{E}_{t-1}\bigg\|\frac{1}{ES}\sum_{k,i\in S} \nabla \cliloss(\param_{i,k-1}) - \nabla \cliloss(\param) + \nabla \cliloss(\param)\bigg\|^2 + \frac{2 \tilde{\eta}^2}{EN} \sum_{k,i}\mathbb{E}_{t-1}\bigg\|\nabla \clilossgm(\param_{i,k-1})  - \nabla \cliloss(\param_{i,k-1})\bigg\|^2
\end{aligned}
\end{equation} 

Again from Eq. \ref{grad_err2} and relaxed triangle inequality (Lemma \ref{relax_tri})

\begin{equation}
\begin{aligned}
\Acal2 & \leq  4 \tilde{\eta}^2 \mathbb{E}_{t-1}\bigg\|\frac{1}{ES}\sum_{k,i\in S} \nabla \cliloss(\param_{i,k-1}) - \nabla \cliloss(\param)\bigg\|^2 + 4 \tilde{\eta}^2 \mathbb{E}_{t-1}\bigg\|\frac{1}{S}\sum_{i\in S}\nabla \cliloss(\param)\bigg\|^2 + 2\tilde{\eta}^2\epsilon_{max}^2\\ 
& \leq  \frac{4 \tilde{\eta}^2}{EN} \sum_{k,i \in N} \mathbb{E}_{t-1}\bigg\| \nabla \cliloss(\param_{i,k-1}) - \nabla \cliloss(\param)\bigg\|^2 + 4 \tilde{\eta}^2 \mathbb{E}_{t-1}\bigg\|\frac{1}{S}\sum_{i\in S}\nabla \cliloss(\param) - \nabla \avgcliloss(\param) + \nabla \avgcliloss(\param)\bigg\|^2 + 2\tilde{\eta}^2\epsilon_{max}^2\\ 
& \leq  \frac{4 \tilde{\eta}^2\beta^2}{EN} \sum_{k,i} \mathbb{E}_{t-1}\bigg\| \param_{i,k-1} - \param\bigg\|^2 + 8 \tilde{\eta}^2\| \nabla \avgcliloss(\param)\|^2 + \bigg( 1 - \frac{S}{N}\bigg)8\tilde{\eta}^2\frac{1}{SN}\sum_i \|\nabla \cliloss(\param)\|^2 + 2\tilde{\eta}^2\epsilon_{max}^2\\ 
&\leq  4 \tilde{\eta}^2\beta^2 \mathcal{E}_t + 16 \tilde{\eta}^2\beta(B^2+1)(\avgcliloss(\param) - \serverloss(\serveroptparam)) + \bigg( 1 - \frac{S}{N}\bigg)\frac{8\tilde{\eta}^2}{S}G^2 +2\tilde{\eta}^2\epsilon_{max}^2\\
\label{A2}
\end{aligned}
\end{equation}

The last step used Assumption (G, B)-BGD assumption  \ref{grad_dis2}. Plugging back the bounds
on $\Acal$1 and $\Acal$2,

\begin{equation}
\begin{aligned}
\mathbb{E}_{t-1}||\param+\Delta \param -\serveroptparam||^2  & = \bigg( 1- \frac{\mu \tilde{\eta}}{2} \bigg)||\param - \serveroptparam||^2 +   2\tilde{\eta}\epsilon_{max} ||\param - \serveroptparam|| - (2\tilde{\eta} - 16 \tilde{\eta}^2\beta(B^2+1))(\avgcliloss(\param) - \serverloss(\serveroptparam)) \\ &+ (1+2\tilde{\eta}\beta)2 \tilde{\eta}\beta \mathcal{E}_t + \bigg( 1 - \frac{S}{N}\bigg)\frac{8\tilde{\eta}^2}{S}G^2 +2\tilde{\eta}^2\epsilon_{max}^2 +\tilde{\eta}^2\sigma^2
\label{eq_con2}
\end{aligned}
\end{equation}

The lemma now follows by observing that $72 \tilde{\eta}^2\beta(B^2+1) \leq 1 $ and that $B \geq 0$.
\end{proof}

\begin{lemma} \label{lem_bd} (bounded drift)  Suppose our functions satisfies assumptions (A1) - (A4).Then the updates of \model\ for any step-size satisfying $\eta_l \leq \frac{1}{(1+B^2)72\beta E\eta_g}$ have bounded drift:

\begin{equation}
\begin{aligned}
3\tilde{\eta}\beta \mathcal{E}_t  \leq   36\beta \tilde{\eta}^3 G^2 + \frac{18\tilde{\eta}^3\beta}{\eta_g^2} \epsilon_{max}^2 + \frac{\beta\tilde{\eta}^3 \sigma^2}{2E\eta_g^2} + \text{\footnotesize$\frac{2\tilde{\eta}}{3}$}(\mathbb{E}[\cliloss(\param^{t-1})]) -\serverloss(\param^*)
\end{aligned}
\end{equation}
\end{lemma}

\begin{proof}

If $E = 1$, the lemma  the lemma trivially holds since $\param_{i,0} = \param$ for all $i \in [N]$ and $\mathcal{E}_t  = 0$. Assume $E \geq 2$ here on. Recall that the local update made on client i is $\param_{i,k} = \param_{i,k-1} - \eta_l \cligradfun (\param_{i,k-1})$. Then,

\begin{equation}
\begin{aligned}
\mathbb{E}\|\param_{i,k} -\param\|^2 &= \mathbb{E}\|\param_{i,k-1} -\param-\eta_l\cligradfun(\param_{i,k-1}) \|^2\\
& \leq \mathbb{E}\|\param_{i,k-1} -\param -\eta_l\cligradfun(\param_{i,k-1})\|^2 + \eta^2_l\sigma^2\\
& = \mathbb{E}\|\param_{i,k-1} -\param -\eta_l(\cligradfun(\param_{i,k-1}) + \nabla \cliloss(\param_{i,k-1}) - \nabla \cliloss(\param_{i,k-1})) \|^2 + \eta^2_l\sigma^2\\
& \leq  2* \mathbb{E}\|\param_{i,k-1} -\param -\eta_l\nabla \cliloss(\param_{i,k-1})\|^2 + 2 \eta_l^2 \| \nabla \clilossgm(\param_{i,k-1})  - \nabla \cliloss(\param_{i,k-1})\|^2 + \eta^2_l\sigma^2\\
\end{aligned}
\end{equation}

Again from Eq. \ref{grad_err2} and relaxed triangle inequality (Lemma \ref{relax_tri})

\begin{equation}
\begin{aligned}
\mathbb{E}\|\param_{i,k} -\param\|^2 & \leq  2 \mathbb{E}\|\param_{i,k-1} -\param -\eta_l\nabla \cliloss(\param_{i,k-1})\|^2 + 2 \eta_l^2 \epsilon_{max}^2 + \eta^2_l\sigma^2\\
& \leq  2(1+\text{\footnotesize$\frac{1}{E-1}$})\mathbb{E}\|\param_{i,k-1} -\param\|^2 + 2E\eta_l^2\|\nabla \cliloss(\param_{i,k-1})\|^2 + 2 \eta_l^2 \epsilon_{max}^2 + \eta^2_l\sigma^2\\
& =  2(1+\text{\footnotesize$\frac{1}{E-1}$})\mathbb{E}\|\param_{i,k-1} -\param\|^2 + \frac{2\tilde{\eta}^2}{\eta_g^2 E}\|\nabla \cliloss(\param_{i,k-1})\|^2 + \frac{2\tilde{\eta}^2}{\eta_g^2 E} \epsilon_{max}^2 + \frac{\tilde{\eta}^2 \sigma^2}{\eta_g^2 E^2}\\
& \leq  2(1+\text{\footnotesize$\frac{1}{E-1}$})\mathbb{E}\|\param_{i,k-1} -\param\|^2 + \frac{4\tilde{\eta}^2}{\eta_g^2 E}\|\nabla \cliloss(\param_{i,k-1}) - \nabla \cliloss(\param)\|^2 \\ \nonumber  &  \quad \quad +\frac{4\tilde{\eta}^2}{\eta_g^2 E}\|\nabla \cliloss(\param)\|^2 + \frac{2\tilde{\eta}^2}{\eta_g^2 E} \epsilon_{max}^2 + \frac{\tilde{\eta}^2 \sigma^2}{\eta_g^2 E^2}\\
& \leq  2(1+\text{\footnotesize$\frac{1}{E-1}$+$\frac{4\tilde{\eta}^2\beta^2}{\eta_g^2 E}$})\mathbb{E}\|\param_{i,k-1} -\param\|^2  + \frac{4\tilde{\eta}^2}{\eta_g^2 E}\|\nabla \cliloss(\param)\|^2 + \frac{2\tilde{\eta}^2}{\eta_g^2 E} \epsilon_{max}^2 + \frac{\tilde{\eta}^2 \sigma^2}{\eta_g^2 E^2}\\
& \leq  2(1+\text{\footnotesize$\frac{2}{E-1}$})\mathbb{E}\|\param_{i,k-1} -\param\|^2  + \frac{4\tilde{\eta}^2}{\eta_g^2 E}\|\nabla \cliloss(\param)\|^2 + \frac{2\tilde{\eta}^2}{\eta_g^2 E} \epsilon_{max}^2 + \frac{\tilde{\eta}^2 \sigma^2}{\eta_g^2 E^2}\\
\end{aligned}
\end{equation}

In the above proof we separated the mean and the variance in the first inequality, then used the relaxed triangle inequality with $a = \text{\footnotesize{$E-1$}}$ in the next inequality. Next equality uses the definition of $\tilde{\eta}$, and the rest follow from the Lipschitzness of the gradient. Unrolling the recursion above,

\begin{equation}
\begin{aligned}
\mathbb{E}\|\param_{i,k} -\param\|^2 & \leq  \sum_{\tau=1}^{k-1}\bigg(\frac{4\tilde{\eta}^2}{\eta_g^2 E}\|\nabla \cliloss(\param)\|^2 + \frac{2\tilde{\eta}^2}{\eta_g^2 E} \epsilon_{max}^2 + \frac{\tilde{\eta}^2 \sigma^2}{\eta_g^2 E^2} \bigg)\bigg( 1+ \frac{2}{E-1}\bigg)^\tau\\
 & \leq  \sum_{\tau=1}^{k-1}\bigg(\frac{4\tilde{\eta}^2}{\eta_g^2 E}\|\nabla \cliloss(\param)\|^2 + \frac{2\tilde{\eta}^2}{\eta_g^2 E} \epsilon_{max}^2 + \frac{\tilde{\eta}^2 \sigma^2}{\eta_g^2 E^2} \bigg)\bigg( 1+ \frac{2}{E-1}\bigg)^\tau\\
  & \leq  \bigg(\frac{4\tilde{\eta}^2}{\eta_g^2 E}\|\nabla \cliloss(\param)\|^2 + \frac{2\tilde{\eta}^2}{\eta_g^2 E} \epsilon_{max}^2 + \frac{\tilde{\eta}^2 \sigma^2}{\eta_g^2 E^2} \bigg)*9E
\end{aligned}
\end{equation}

Averaging over $i$ and $k$, multiplying by $3\tilde{\eta}\beta$ and then using Assumption A1,

\begin{equation}
\begin{aligned}
3\tilde{\eta}\beta \mathcal{E}_t & \leq  \frac{1}{N} \sum_i 108\beta \tilde{\eta}^3\|\nabla \cliloss(\param)\|^2 + \frac{54\tilde{\eta}^3\beta}{\eta_g^2} \epsilon_{max}^2 + \frac{27\beta\tilde{\eta}^3 \sigma^2}{\eta_g^2 E} \\
& \leq   108\beta \tilde{\eta}^3 G^2 + \frac{54\tilde{\eta}^3\beta}{\eta_g^2} \epsilon_{max}^2 + \frac{27\beta\tilde{\eta}^3 \sigma^2}{\eta_g^2 E} + 216\tilde{\eta}^3\beta^2B^2(\avgcliloss(\param) - \serverloss
(\serveroptparam))
\end{aligned}
\end{equation}

The lemma now follows from our assumption that $72 \tilde{\eta}^2\beta(B^2+1) \leq 1 $.

\end{proof}

\begin{theorem}
Adding the statements of Theorem \ref{lem_one} and Lemma \ref{lem_bd}, we get

\begin{equation}
\begin{aligned}
\mathbb{E}||\param^t -\serveroptparam||^2  & \leq \bigg( 1- \frac{\mu \tilde{\eta}}{2} - 2\tilde{\eta}\epsilon_{max}\bigg)\mathbb{E}||\param^{t-1} - \serveroptparam||^2 +\tilde{\eta}^2\sigma^2 + \bigg( 1 - \frac{S}{N}\bigg)\frac{8\tilde{\eta}^2}{S}G^2 +2\tilde{\eta}^2\epsilon_{max}^2 \\
&- \tilde{\eta}(\mathbb{E}[\avgcliloss(\param^{t-1})] - \serverloss(\serveroptparam)) +  108\beta \tilde{\eta}^3 G^2 + \frac{54\tilde{\eta}^3\beta}{\eta_g^2} \epsilon_{max}^2 + \frac{27\beta\tilde{\eta}^3 \sigma^2}{\eta_g^2 E} + \text{\footnotesize$2\tilde{\eta}$}(\mathbb{E}[\avgcliloss(\param^{t-1})]) -\serverloss(\serveroptparam) \\
\\
& = \bigg( 1- \frac{\mu \tilde{\eta}}{2} - 2\tilde{\eta}\epsilon_{max}\bigg)\mathbb{E}||\param - \serveroptparam||^2 + \tilde{\eta}\bigg(\mathbb{E}[\avgcliloss(\param^{t-1})] -\serverloss(\serveroptparam)\bigg) + 2\tilde{\eta}^2\bigg(1 + \frac{27\tilde{\eta}\beta}{\eta_g^2}\bigg)\epsilon_{max}^2 \\
& +\tilde{\eta}^2\bigg( \sigma^2\bigg( 1 + \frac{27\beta\tilde{\eta}^3 \sigma^2}{\eta_g^2 E}\bigg) + \bigg( 1 - \frac{S}{N}\bigg)\frac{8\tilde{\eta}^2}{S}G^2  +  36\beta \tilde{\eta}^3 G^2\bigg) \\
\end{aligned}
\end{equation}
\label{thm:convergence-result}
\end{theorem}

\section{Datasets Details}
In table \ref{tab:textdatasplits} we list the details about the datasets used in the experiments. The table shows the numbert of classes, split proportions of dataset across clients and server. To highlight the \noniid partition across clients, we show a heatmap  in the Figure \ref{fig:clinetDis}.

\begin{table}[h]
    \centering
    \resizebox{0.9\textwidth}{!}{
    \begin{tabular}{|l|c|c|c|c|c|}
    \hline
    \hline
        Dataset & \#Classes $(|\Ycal|)$  & \#Clients' data $(| \bigcup_{i =1}^N D_i|)$ & \#Server's data $(|\valdata|)$ & \#Test $(|D_{\text{Test}}|)$ \\ \hline \hline
        Flowers & 5   & 3270  & 200  & 200    \\ \hline
        FEMNIST &  10  & 60000  & 5000   & 5000    \\ \hline
        CIFAR10 & 10 &   50000  & 5000   & 5000   \\ \hline
        CIFAR100 & 100 & 50000  & 5000   & 5000    \\ \hline
        \hline
    \end{tabular}}
    \caption{Dataset statistics} 
    \label{tab:textdatasplits}
\end{table}

\begin{figure}[h]
\centering
%\hspace{-0.6cm}
\begin{subfigure}[b]{0.35\linewidth}
\centering
\includegraphics[width=\linewidth]{IJCAI/new_figure/data distribution/flowers.pdf}
\caption*{$\underbracket[1pt][1.0mm]{\hspace{5cm}}_{\substack{\vspace{-4.0mm}\\
\colorbox{white}{(a) \scriptsize FLOWERS}}}$}
\phantomcaption
%\label{fig:CIFAR100}

\end{subfigure}
\begin{subfigure}[b]{0.35\linewidth}
\centering
\includegraphics[width=\linewidth]{IJCAI/new_figure/data distribution/femnist.pdf}
\caption*{$\underbracket[1pt][1mm]{\hspace{5cm}}_{\substack{\vspace{-4.0mm}\\
\colorbox{white}{(b) \scriptsize FEMNIST}}}$}
\phantomcaption
%\label{fig:CIFAR10}
\end{subfigure}

%\hspace{-0.6cm}
\begin{subfigure}[b]{0.35\linewidth}
\centering
\includegraphics[width=\linewidth]{IJCAI/new_figure/data distribution/cifar_10.pdf}
\caption*{$\underbracket[1pt][1.0mm]{\hspace{5cm}}_{\substack{\vspace{-4.0mm}\\
\colorbox{white}{(a) \scriptsize CIFAR10}}}$}
\phantomcaption
%\label{fig:CIFAR100}

\end{subfigure}
\begin{subfigure}[b]{0.35\linewidth}
\centering
\includegraphics[width=\linewidth]{IJCAI/new_figure/data distribution/cifar_100.pdf}
\caption*{$\underbracket[1pt][1mm]{\hspace{5cm}}_{\substack{\vspace{-4.0mm}\\
\colorbox{white}{(b) \scriptsize CIFAR100}}}$}
\phantomcaption
%\label{fig:CIFAR10}
\end{subfigure}
\caption{Classwise distribution of training instances across clients. The X axis spans the clients and the Y axis spans the classes. Each rectangle represents the number of instances that belong to a particular a class in a client. A dark rectangle in the cell $(i, j)$ means that the $i^{\text{th}}$ client has more instances of class $j$.}
\label{fig:clinetDis}
\end{figure}

\section{Additional experiments}

\subsection{Ablation study: Varying Budget $b$} All coreset selection algorithms' performances are affected by the size of the subset they are allowed to select. We present the effect of varying the sampling budget on coreset selection algorithms under $40\%$ close-set noise in Figure \ref{fig:bugdet_experiments}. For a fair comparison we make the number of SGD steps consistent across different sampling budgets. For CIFAR10, in Figure \ref{fig:bugdet_experiments} a) we see that \model{}'s performance is robust to sampling budget and other coreset methods slightly improve as budget size increases. We attribute this robustness to the fact that \model{} selects coreset based on label-wise last layer server gradients. However, for CIFAR100 dataset, in Figure \ref{fig:bugdet_experiments} b) we see all the methods improve with increase in the budget size, since it is slightly a more difficult dataset having $100$ classes. 

 %\resizebox{0.9\textwidth}{!}{
\begin{figure}[h]
\centering
%\begin{minipage} {0.7\textwidth}
%\includegraphics[width =0.8\linewidth,trim={.25cm .5cm 0 0},clip] {AAAI/new_figures/Legend_val_one_line.pdf}
\includegraphics[width =0.15\linewidth] {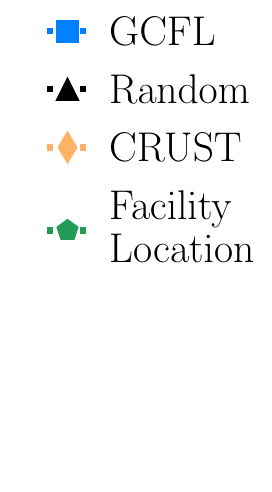}
\centering
%\hspace{-0.6cm}
\begin{subfigure}[b]{0.30\linewidth}
\centering
\includegraphics[width=\linewidth]{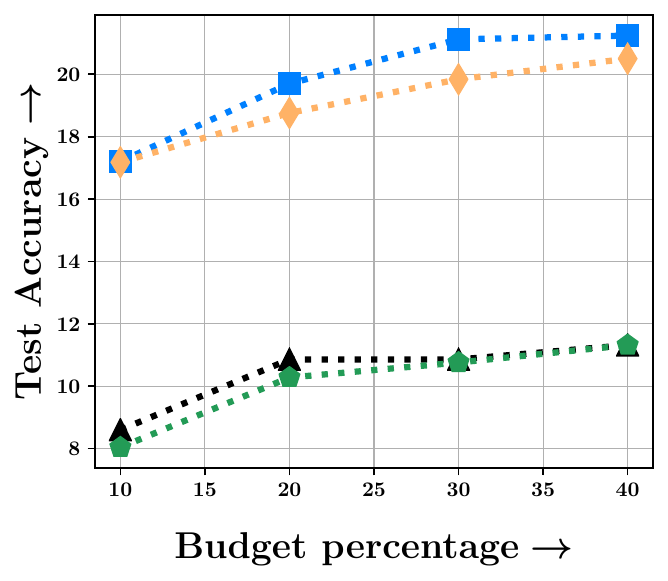}
\caption*{$\underbracket[1pt][1.0mm]{\hspace{4.7cm}}_{\substack{\vspace{-4.0mm}\\
\colorbox{white}{(a) \scriptsize CIFAR100}}}$}
\phantomcaption
%\label{fig:CIFAR100}

\end{subfigure}
\begin{subfigure}[b]{0.3\linewidth}
\centering
\includegraphics[width=\linewidth]{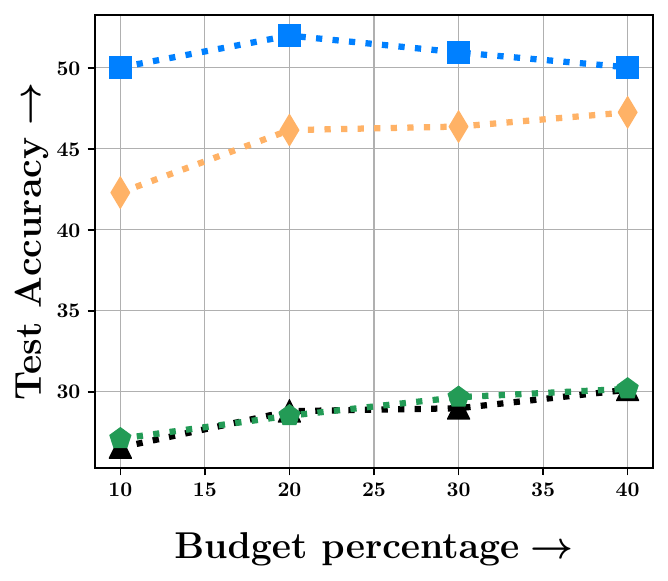}
\caption*{$\underbracket[1pt][1mm]{\hspace{4.7cm}}_{\substack{\vspace{-4.0mm}\\
\colorbox{white}{(b) \scriptsize CIFAR10}}}$}
\phantomcaption
%\label{fig:CIFAR10}
\end{subfigure}
\caption{Performance of \model\ and other subset selection method as we vary budget in 40\% closeset noise setting.}
\label{fig:bugdet_experiments}
%\end{minipage}
\end{figure}

%\begin{minipage} {0.7\textwidth}
\begin{figure}[h]
\centering
\includegraphics[width =0.15\linewidth] {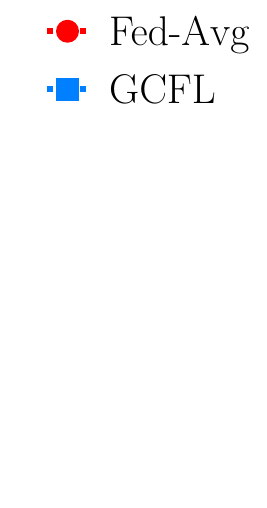}
\centering
%\hspace{-0.6cm}
\begin{subfigure}[b]{0.3\linewidth}
\centering
\includegraphics[width=\linewidth]{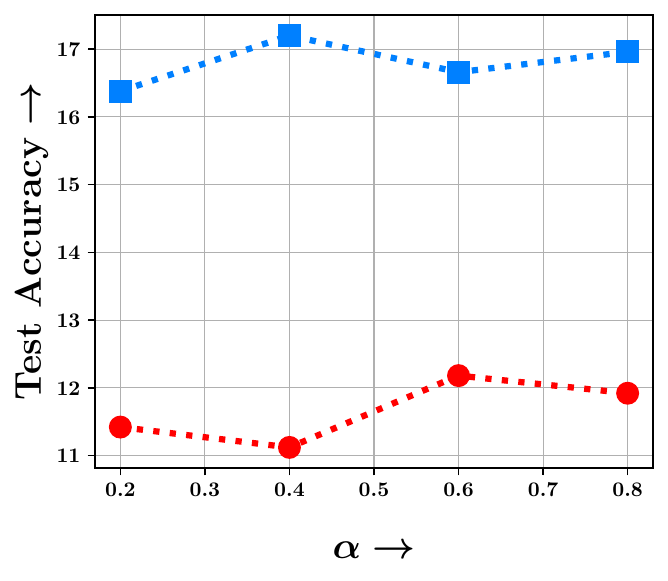}
\caption*{$\underbracket[1pt][1.0mm]{\hspace{4.7cm}}_{\substack{\vspace{-4.0mm}\\
\colorbox{white}{(a) \scriptsize CIFAR100}}}$}
\phantomcaption
%\label{fig:CIFAR100}

\end{subfigure}
\begin{subfigure}[b]{0.3\linewidth}
\centering
\includegraphics[width=\linewidth]{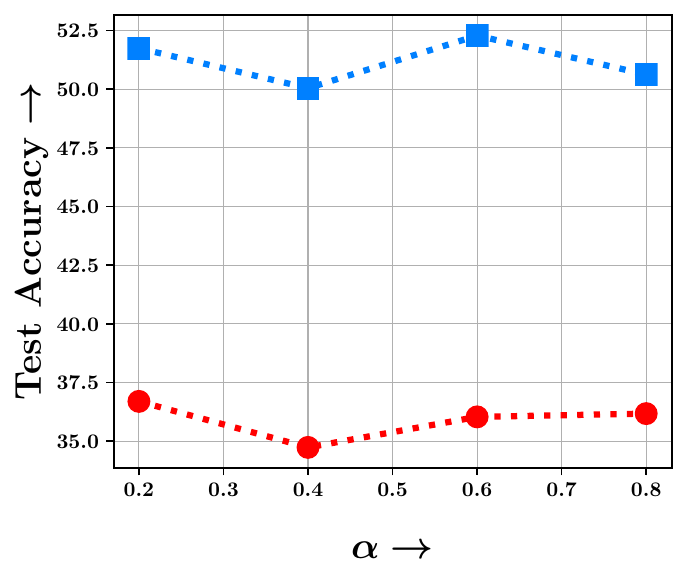}
\caption*{$\underbracket[1pt][1mm]{\hspace{4.7cm}}_{\substack{\vspace{-4.0mm}\\
\colorbox{white}{(b) \scriptsize CIFAR10}}}$}
\phantomcaption
%\label{fig:CIFAR10}
\end{subfigure}
\caption{Performance of \model\ and Federated averaging as we vary $\alpha$(parameter controlling non-IID split among clients) in 40\% closeset noise setting.}
\label{fig:alpha_experiments}
%\end{minipage}
\end{figure}

%\newpage

\subsection{Ablation study: Varying Non-IIDness among clients $\alpha$}
We distributed the data to clients following \citep{fedem} where we simulate the \noniid data partition by sampling class proportions from a symmetric Dirichlet Distribution parameterized with $\alpha$. Typically, setting a lesser $\alpha$ would result in a very skewed class proportion across clients and as $\alpha$ increases we reach the uniform partition (\iid) in the limit. We conduct experiments under the closed set label noise with a noise ratio of $40\%$ to assess the performance of \model{} as against to the standard Federated Averaging algorithm. The results are presented in the Figure \ref{fig:alpha_experiments} which clearly elucidate the robustness of \model{} primarily attributes to its ability to balance the coreset across classed by deliberately running the selection on a per-class basis alongside selecting noise-free informative points. On the otherhand, Federated averaging, due to its sensitivity to noise, is unable to recover even when the partition reflectds \iid characteristics.

% \begin{table}[t]
%     \centering
%     \begin{tabular}{|c|c|c|c|c|}
%     \hline
%         \multirow{2}{3em}{Method} &\multicolumn{2}{c|}{CIFAR10} & \multicolumn{2}{c|}{CIFAR100}\\ \cline{2-5}
%          & \#rounds  & speedup & \#rounds  &  speedup      \\ \hline
%         FedAvg &  & 1x &   & 1x       \\ \hline        
%         \hline
%     \end{tabular}
%     \caption{} 
%     \label{tab:textdatasplits}
% \end{table}
